# Supplementary material for: A nested sampling code for targeted searches for continuous gravitational waves from pulsars
Source: arXiv:1705.08978 source file (2017-05-24)
Supplement: Supplementary file 1 [file caption.tex]

\label{fig:approx_odds}
The upper plot shows coherent signal-to-noise ratio ($\rho_{\text{coh}}$) versus the logarithm of odds for
two different cases: coherent signal versus Gaussian noise $\mathcal{O}_{\text{S}}/{\text{N}}$ and coherent signal versus
incoherent signal $\mathcal{O}_{\text{S}/\text{I}_{\text{simple}}}$. In both cases, and for each $\rho_{\text{coh}}$, there are values for
100 realisations of noise, with the median and maximum values, for $\mathcal{O}_{\text{S}}/{\text{N}}$ and $\mathcal{O}^S_I$
respectively, highlighted with larger points. Overplotted are the approximate values expected for these two
odds. The lower plot just shows $\mathcal{O}^S_I$ to make its relation to $\rho_{\text{coh}}$ more obvious.
